# Supplementary material for: RDRN: Recursively Defined Residual Network for Image Super-Resolution
Source: arXiv:2211.09462 source file (2022-11-17)
Supplement: Supplementary file 2 [file title_supp.tex]

%\title{Supplementary for \model: \modelfullnametitle{}  for Image Super-Resolution}
%\author{
%	Alexander Panaetov, Karim Daou, Igor Samenko, Evgeny Tetin, Ilya Ivanov  \\
%	\small Intelligent systems and Data science Technology center \\
%	\small`Huawei Technologies Co., Ltd
%}

\title{Supplementary for \model: \modelfullnametitle{}  for Image Super-Resolution}
